# Supplementary material for: Real-Time Propagation TDDFT and Density Analysis for Exciton Couplings Calculations in Large Systems
Source: arXiv:1902.10583 ancillary file (2019-05-16)
Supplement: Supplementary file 1 [file jjs_il_ptddft_si.pdf]

# Real-Time Propagation TDDFT and Density Analysis for Exciton Coupling Calculations in Large Systems

Joaquim Jornet-Somoza<sup>\*,†,‡</sup> and Irina Lebedeva<sup>†</sup>

<sup>†</sup>*Nano-Bio Spectroscopy Group and ETSF Scientific Development Centre, Department of Materials Physics, University of the Basque Country, CFM CSIC-UPV/EHU-MPC and DIPC, Tolosa Hiribidea 72, E-20018 Donostia-San Sebastián*

<sup>‡</sup>*Theory Department, Max Planck Institute for the Structure and Dynamics of Matter and Center for Free-Electron Laser Science, Luruper Chaussee 149, 22761 Hamburg, Germany*

E-mail: j.jornet.somoza@gmail.com

## 1 Computational Details

The quantum chemistry/physics code `OCTOPUS` is a real-space TDDFT software designed to perform time-propagation calculations. The code is highly parallelized in space domains for evaluation of the Hamiltonian used, as well as in Kohn-Sham states for the time propagation. These features make `OCTOPUS` the ideal code for the implementation of our method to compute the excitation coupling between different molecules.

The benzaldehyde molecule geometry has been optimized using ORCA at the DFT level using the exchange Becke88<sup>1</sup> and correlation Perdew86<sup>2</sup> (BP86) GGA functionals, the atom-pairwise dispersion correction with the Becke-Johnson damping scheme (D3BJ)<sup>3,4</sup> and the contracted split valence plus polarization basis set def2-SVP.<sup>5</sup> The resolution of the identity

(RI-J) approximation for the Coulomb potential<sup>6</sup> is applied with the def2/J auxiliary basis set.<sup>7</sup> The optimized geometry is then used for the generation of supramolecular systems, i.e. dimer and cluster geometries.

ORCA package is used to compute excited states within linear-response TDDFT solving the full Casida's equation. Usually excited states calculations require the use of an extended basis set and augmented diffuse functions. We apply the ma-def2-TVZP basis set<sup>5,8</sup> and the def2/J auxiliary basis set for the RI approximation. For these calculation, we use the Perdew, Burke and Ernzerhof (PBE) exchange-correlation functional.<sup>9,10</sup>

The time-propagation TDDFT calculations are performed with the OCTOPUS code. The real-space grid is defined by the minimum mesh formed by spheres of the radius of 4.5 Å centered around each atom (except for the isolated molecule study, where we use the radius of 6.0 Å) and the spacing between grid points of 0.18 Å. To make the calculations computationally affordable, the core electrons are treated with norm-conserving Troullier-Martins pseudopotentials. For the calculation of absorption spectra, three different time-propagation runs are carried out starting from the ground state wave function. In each of these simulations, the system is perturbed by a delta kick of the electric dipole potential polarized along one of the Cartesian axes. The strength of this external electric field is set to  $0.01 \text{ Å}^{-1}$ . The electronic time propagations are performed for the total propagation time of  $\tau = 40 \text{ fs}$  with the time step of  $dt \approx 1.49 \text{ as}$ . These parameters ensure the spectral resolution of  $dw \approx 0.1 \text{ eV}$ . The absorption spectra are generated from the Fourier transform of the dynamic polarizability using the Gaussian damping that ensures that the function acquires the value equal to  $10^{-4}$  at the end of the propagation time. This values causes a broadening of excitation peaks of  $\approx 0.083 \text{ eV}$  at the half maximum (see section below for the detailed description and derivation).

As described in the main text, the local density domains around each molecule are determined as argued by the "Quantum Theory of Atoms in Molecules" developed by R.F.W. Bader. In particular, the electronic density belonging to each molecule is found following the

gradient paths until reaching atoms of the molecule, where the density becomes maximum. We have implemented this procedure in the recent version of the **OCTOPUS** code.

We have also implemented in **OCTOPUS** the utility for Fourier transformation of time-dependent electronic densities necessary for computing transition densities. The calculation of excitation couplings is also implemented in a local repository and will be soon available in the development version of the **OCTOPUS** code.

## 2 Damping factor effect on the peak broadening

As explained in the main text, the practical implementation of equation (4) in the main text requires the addition of a damping function to remove spurious peaks. We use the Gaussian function with the damping parameter  $\eta$  that ensures that the this function achieves the value of  $10^{-4}$  at the end of the propagation time:

$$D(t) = e^{-\eta^2 t^2}, \quad (\text{S1})$$

$$\eta = \frac{\sqrt{-\ln(1e^{-4})}}{\tau}. \quad (\text{S2})$$

Then, the dynamic polarizability is obtained using

$$\alpha_{\nu\lambda}(\omega) = \frac{1}{k_\lambda} \int_0^\tau dt [\mu_\nu(t) - \mu_\nu(0)] e^{-i\omega t} e^{-\eta^2 t^2}. \quad (\text{S3})$$

Fourier transformation of this expression now involves the Fourier transformation of the damping function:

$$\mathcal{F}_t[D](\omega) = \frac{1}{\eta\sqrt{2}} e^{-\frac{(\omega)^2}{4\eta^2}}, \quad (\text{S4})$$

$$\sigma_{hwhm} = 2\sqrt{\ln 2} \cdot \eta, \quad (\text{S5})$$

where  $\sigma_{hwhm}$  is the half-weight at half-maxima (HWHM) of the Gaussian function, and the

Fourier Transform pair of a function  $f(x)$  is defined through equations  $\mathcal{F}_x(k) = \frac{1}{\sqrt{2\pi}} \int_{-\infty}^{\infty} f(x) e^{ikx}$  and  $f(x) = \frac{1}{\sqrt{2\pi}} \int_{-\infty}^{\infty} \mathcal{F}_x(k) e^{-ikx}$ .

Let us now determine which broadening acquires the spectral function due to the damping function. Looking at equations (7) in the main text and (S4), we see the following proportionality:

$$\mathcal{F}[Tr(\Im m(\boldsymbol{\alpha}(t)))] \propto \sum_{n=1}^{\Omega_n} \delta(\omega - \Omega_n), \quad (\text{S6a})$$

$$\mathcal{F}[D(t)] \propto G(\omega). \quad (\text{S6b})$$

where  $G$  is the normalized Gaussian function characterized by its HWHM value,  $\sigma_{hwhm}$ .

Using the convolution theorem, we see that the convolution of the delta function with the Gaussian function gives just a displacement of the Gaussian function,

$$\mathcal{F}[Tr(\Im m(\boldsymbol{\alpha}(t))D(t))] = \mathcal{F}[Tr(\Im m(\boldsymbol{\alpha}(t)))] * \mathcal{F}[D(t)] \propto \sum_{n=1}^N G(\omega - \Omega_n). \quad (\text{S7})$$

### 3 Supplementary Figures

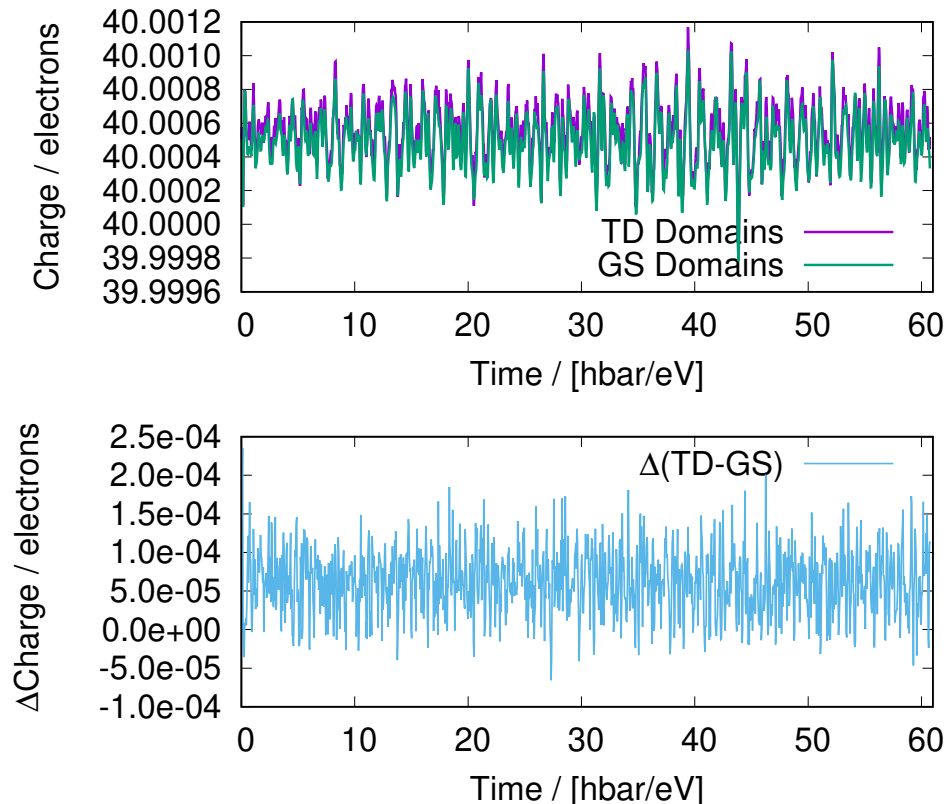

Figure S 1: Charge density evolution during a P-TDDFT run for one benzaldehyde molecule in a dimer with the molecules separated by 4 Å in the  $z$  direction for the electric field polarized along the  $y$  direction. Since we use the sg15 pseudopotential, the ground state (GS) charge corresponding to valence electrons for one benzaldehyde molecule is 40 electrons. The maximum oscillation of the charge corresponds to 0.0012 electrons, i.e. a 0.005%. GS Domains refers to the electron charge inside the domain determined for the GS density, while for the TD Domains, the local charge analysis is performed at each time step stored. The difference between two values is always smaller than 0.00025 electrons.

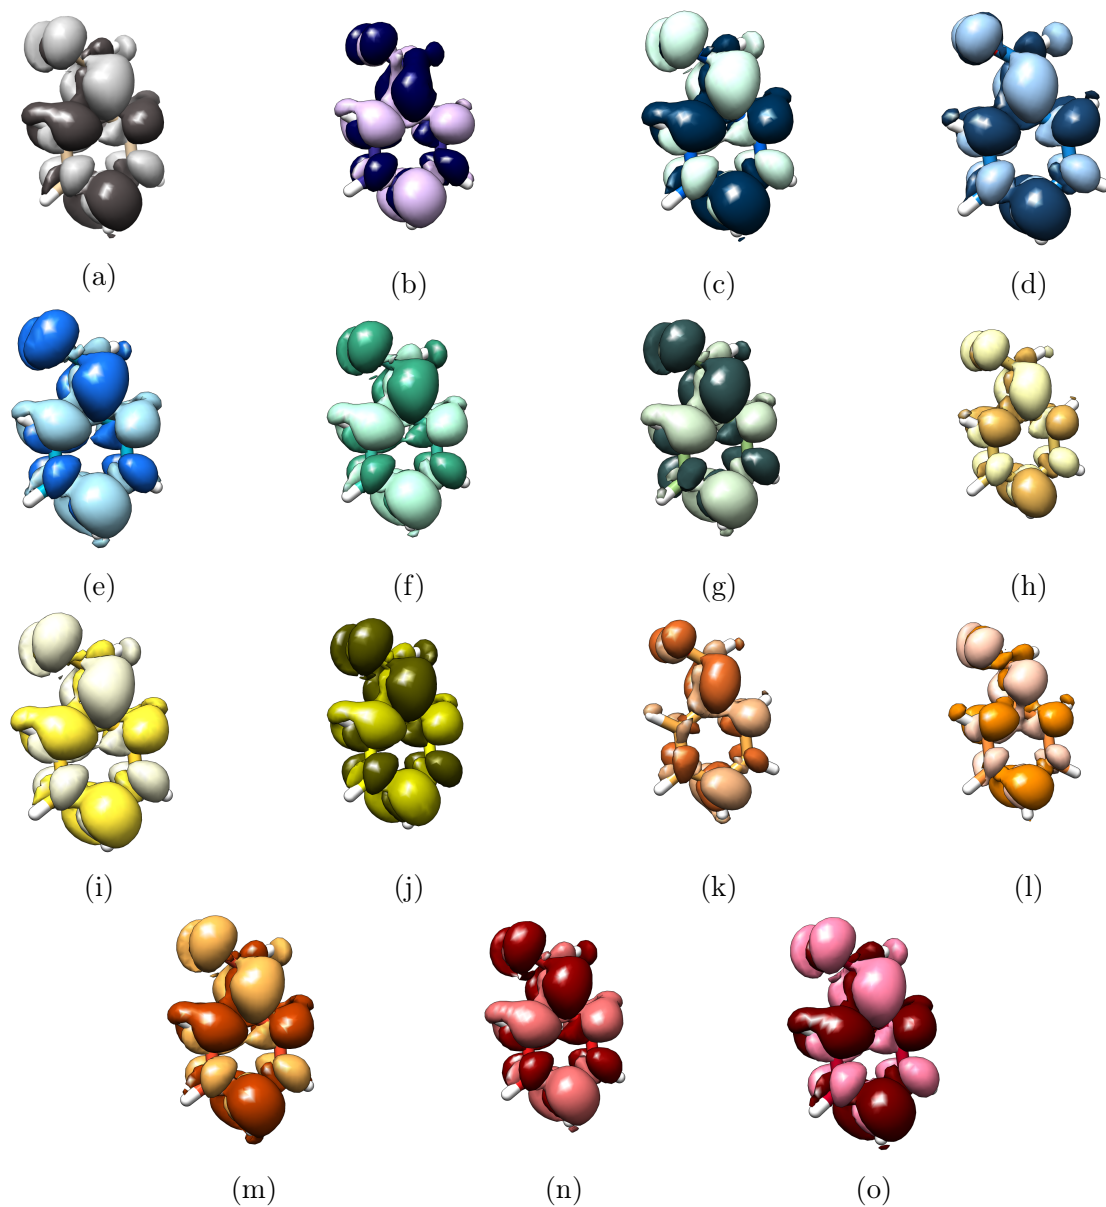

Figure S 2: (S2a) Transition density corresponding to the  $3^1A' \leftarrow 0$  transition for the isolated molecule. (S2b-S2o) Transition densities of benzaldehyde molecules in the cluster for the main excitation peak below 5 eV corresponding to the  $3^1A' \leftarrow 0$  transition (isosurface  $0.0075 \text{ \AA}^{-3}$ ). The color sequence correlates with the colors used in Figure 6 in the main text.

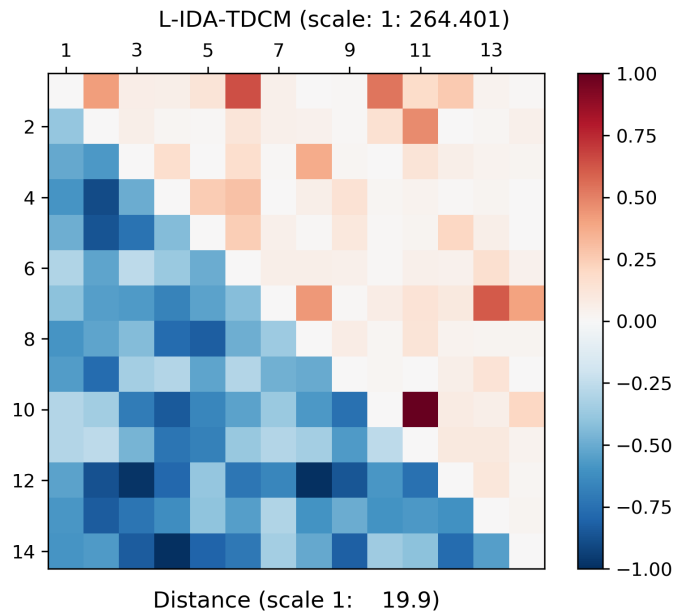

Figure S 3: Map of the exciton coupling between benzaldehyde molecules in the cluster. Labels correspond to Figure 6a. The up-diagonal part (red) shows the difference between the exciton coupling computed using the transition density cube method (TDCM) and in the ideal dipole approximation (IDA) with the transition dipole moment obtained by fitting the dynamic polarizability for each local charge density (LDT). The absolute values are rescaled by the maximum difference found and expressed in parenthesis in wavenumber units ( $\text{cm}^{-1}$ ). The low-diagonal part (blue) represents the inter-molecular distance. The absolute values are rescaled by the maximum distance found and expressed in parenthesis in Angstrom units ( $\text{\AA}$ ).

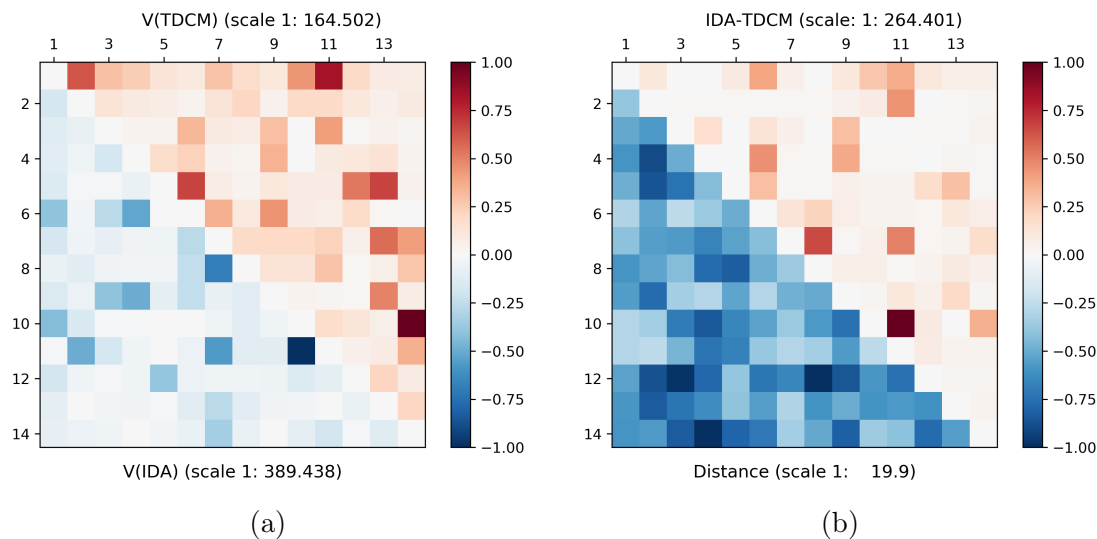

Figure S 4: Map of the exciton coupling between benzaldehyde molecules in the cluster. Labels correspond to Figure 6a. (S4a) The up-diagonal part (red) shows the exciton coupling computed using the transition density cube method (TDCM), while the low-diagonal part (blue) is computed in the ideal dipole approximation (IDA) with the transition dipole moment of one isolated benzaldehyde molecule (IM). The absolute values are rescaled by the maximum found for each method and expressed in parenthesis in wavenumber units ( $\text{cm}^{-1}$ ). (S4b) The up-diagonal part (red) corresponds to the difference between the exciton coupling computed using the TDCM method and IDA-IM. The absolute values are rescaled by the maximum difference found and expressed in parenthesis in wavenumber units ( $\text{cm}^{-1}$ ). The low-diagonal part (blue) represents the inter-molecular distance. The absolute values are rescaled by the maximum distance found and expressed in parenthesis in Angstrom units ( $\text{\AA}$ ).

## 4 Supplementary Tables

Table S 1: Comparison of several ground-state eigenvalues (in eV) between the results obtained using the real-space grid (OCTOPUS) and localized atomic orbitals (ORCA). HOMO and LUMO refer to the high occupied and low unoccupied molecular orbital, respectively. The grid used in OCTOPUS is defined by spheres of radius 6 Å and spacing between the points of 0.16 Å. The basis set used in the ORCA calculations is the contracted basis set ma-def2-TZVP.<sup>5,7,8</sup>

| Molecular Level | OCTOPUS         | ORCA                      |
|-----------------|-----------------|---------------------------|
|                 | real-space grid | localized atomic orbitals |
| HOMO-3          | -8.6524         | -8.6246                   |
| HOMO-2          | -6.8793         | -6.8621                   |
| HOMO-1          | -6.7969         | -6.7799                   |
| HOMO            | -5.9734         | -5.9588                   |
| LUMO            | -2.9816         | -2.9480                   |
| LUMO+1          | -1.7735         | -1.7417                   |
| LUMO+2          | -0.5967         | -0.5505                   |
| LUMO+3          | -0.5681         | -0.5491                   |

Table S 2: Reoriented transition dipole moments for the  $3^1A' \leftarrow 0$  excitation of benzaldehyde molecules in the cluster obtained from the transition dipole moment of the isolated molecule (IM).

| Label | $\epsilon(3^1A') / \text{eV}$ | $\mu_x / \text{\AA}$ | $\mu_y / \text{\AA}$ | $\mu_z / \text{\AA}$ |
|-------|-------------------------------|----------------------|----------------------|----------------------|
| 1     | 4.78                          | -0.0098              | -1.3783              | 0.1776               |
| 2     | 4.78                          | -0.5444              | -0.0297              | -1.2783              |
| 3     | 4.78                          | 0.9039               | 0.0055               | 1.0556               |
| 4     | 4.78                          | -1.0592              | 0.5706               | 0.6956               |
| 5     | 4.78                          | 1.0208               | -0.9426              | 0.0279               |
| 6     | 4.78                          | 0.9347               | -0.4129              | 0.9418               |
| 7     | 4.78                          | -0.5710              | -0.8309              | 0.9564               |
| 8     | 4.78                          | -0.6981              | 0.6185               | -1.0302              |
| 9     | 4.78                          | -1.1502              | 0.7648               | 0.1528               |
| 10    | 4.78                          | 0.8254               | -0.1992              | -1.1001              |
| 11    | 4.78                          | 0.2703               | -0.5444              | 1.2497               |
| 12    | 4.78                          | 0.3723               | -1.0771              | 0.7953               |
| 13    | 4.78                          | 0.4017               | -1.1673              | 0.6382               |
| 14    | 4.78                          | 0.3666               | -1.2260              | 0.5419               |

Table S 3: Transition dipole moments of benzaldehyde molecules in the cluster for the main excitation peak below 5 eV computed from the Gaussian fit and diagonalization of the dynamic polarizability tensor (LDT).

| Label | $\epsilon(3^1A')$ /eV | $\mu_x$ / Å | $\mu_y$ / Å | $\mu_z$ / Å |
|-------|-----------------------|-------------|-------------|-------------|
| 1     | 4.77                  | 0.0266      | -0.5579     | 0.0247      |
| 2     | 4.77                  | 0.2024      | -0.0093     | 0.6587      |
| 3     | 4.93                  | -0.1856     | 0.4075      | 0.2034      |
| 4     | 4.73                  | -0.6661     | 0.1066      | -0.0641     |
| 5     | 4.76                  | -0.2347     | -0.0419     | -0.6937     |
| 6     | 4.73                  | -0.3999     | -0.4336     | 0.2609      |
| 7     | 4.66                  | 0.4185      | 0.2295      | -0.2002     |
| 8     | 4.80                  | 0.1992      | 0.4691      | 0.4749      |
| 9     | 4.80                  | -0.6338     | -0.2158     | 0.0737      |
| 10    | 4.77                  | -0.2081     | -0.2351     | -0.3186     |
| 11    | 4.34                  | -0.0105     | 0.4355      | -0.0970     |
| 12    | 4.76                  | -0.0889     | 0.5971      | -0.4433     |
| 13    | 4.75                  | 0.5147      | -0.4065     | 0.2970      |
| 14    | 4.78                  | -0.6536     | 0.1830      | -0.1261     |

Table S 4: Transition dipole moments of benzaldehyde molecules in the cluster for the main excitation peak below 5 eV computed from the transition density as defined in equation 20.

| Label | $\epsilon(3^1A')$ /eV | $\mu_x$ / Å | $\mu_y$ / Å | $\mu_z$ / Å | $\Delta \mu _{TDCM}^{LDT}$ / Å | Twist / ° |
|-------|-----------------------|-------------|-------------|-------------|--------------------------------|-----------|
| 1     | 4.77                  | -0.0658     | 0.5628      | -0.1024     | 0.0167                         | 8.6396    |
| 2     | 4.77                  | -0.2729     | -0.0109     | -0.6597     | 0.0248                         | 5.6426    |
| 3     | 4.93                  | 0.1453      | -0.4332     | -0.2194     | 0.0151                         | 5.5251    |
| 4     | 4.73                  | 0.6793      | -0.1425     | 0.0315      | 0.0172                         | 3.9378    |
| 5     | 4.76                  | 0.2188      | 0.0388      | 0.6947      | 0.0041                         | 1.2288    |
| 6     | 4.73                  | 0.4617      | 0.4478      | -0.2114     | 0.0320                         | 6.3991    |
| 7     | 4.66                  | -0.4258     | -0.1706     | 0.0470      | 0.0564                         | 18.1737   |
| 8     | 4.80                  | -0.2100     | -0.4681     | -0.4691     | 0.0014                         | 1.0082    |
| 9     | 4.80                  | 0.6385      | 0.2481      | -0.0752     | 0.0155                         | 2.4176    |
| 10    | 4.77                  | 0.1193      | 0.2061      | 0.3283      | 0.0417                         | 11.3373   |
| 11    | 4.34                  | -0.0301     | -0.4409     | 0.1051      | 0.0080                         | 5.2234    |
| 12    | 4.76                  | 0.0692      | -0.5934     | 0.4625      | 0.0065                         | 2.0565    |
| 13    | 4.75                  | -0.5239     | 0.3991      | -0.2291     | 0.0227                         | 5.2637    |
| 14    | 4.78                  | 0.6526      | -0.2319     | 0.1201      | 0.0125                         | 3.9217    |

Table S 5: Exciton coupling between benzaldehyde molecules of the cluster (in  $\text{cm}^{-1}$ ). Labels correspond to Figure 6a. The up-diagonal part (red) corresponds to the exciton coupling computed using the transition density cube method (TDCM), while the low-diagonal part (blue) is obtained in the ideal dipole approximation (IDA) using the transition dipole moment of one isolated benzaldehyde molecule (IM).

| Labels | 1      | 2      | 3      | 4      | 5      | 6      | 7      | 8     | 9     | 10     | 11     | 12    | 13     | 14     |
|--------|--------|--------|--------|--------|--------|--------|--------|-------|-------|--------|--------|-------|--------|--------|
| 1      |        | 104.10 | 48.73  | 40.97  | 21.08  | 15.83  | 47.24  | 29.23 | 17.71 | 72.05  | 136.50 | 31.45 | 12.91  | 12.22  |
| 2      | 65.39  |        | 22.08  | 14.24  | 12.26  | 5.48   | 20.89  | 34.21 | 7.06  | 31.22  | 31.46  | 17.25 | 8.38   | 14.90  |
| 3      | 47.40  | 27.52  |        | 5.93   | 6.34   | 55.25  | 14.83  | 12.73 | 49.75 | 1.23   | 69.30  | 1.96  | 6.87   | 4.95   |
| 4      | 40.42  | 17.33  | 67.26  |        | 29.10  | 37.61  | 7.01   | 4.73  | 56.77 | 1.07   | 14.72  | 16.89 | 23.25  | 6.31   |
| 5      | 52.07  | 5.53   | 6.04   | 26.62  |        | 110.73 | 12.28  | 6.35  | 17.51 | 13.36  | 13.47  | 86.29 | 111.23 | 7.10   |
| 6      | 158.14 | 9.44   | 105.33 | 202.97 | 1.11   |        | 57.98  | 16.30 | 73.76 | 13.58  | 10.84  | 30.35 | 2.62   | 1.15   |
| 7      | 66.21  | 17.90  | 32.66  | 13.49  | 17.75  | 105.74 |        | 31.02 | 32.83 | 32.38  | 37.78  | 8.48  | 92.00  | 69.26  |
| 8      | 27.00  | 40.34  | 12.50  | 10.92  | 11.71  | 96.85  | 269.16 |       | 22.40 | 21.08  | 47.02  | 3.63  | 9.20   | 45.14  |
| 9      | 57.10  | 23.71  | 157.73 | 194.21 | 35.36  | 97.12  | 29.85  | 43.05 |       | 6.42   | 4.06   | 2.97  | 81.49  | 12.57  |
| 10     | 168.45 | 59.73  | 3.71   | 5.09   | 0.34   | 1.46   | 15.46  | 43.59 | 17.47 |        | 28.93  | 19.87 | 9.61   | 164.50 |
| 11     | 3.11   | 194.45 | 69.21  | 18.01  | 1.55   | 24.15  | 220.19 | 43.43 | 42.34 | 389.44 |        | 7.94  | 13.83  | 58.73  |
| 12     | 72.01  | 17.79  | 5.93   | 16.84  | 149.78 | 23.17  | 16.56  | 15.76 | 20.22 | 52.02  | 37.57  |       | 34.90  | 13.46  |
| 13     | 34.65  | 1.64   | 9.82   | 12.80  | 6.01   | 40.71  | 105.99 | 40.94 | 13.41 | 9.77   | 1.59   | 26.17 |        | 34.70  |
| 14     | 33.17  | 23.67  | 16.84  | 0.79   | 11.76  | 24.76  | 132.39 | 27.09 | 1.56  | 37.17  | 70.33  | 4.86  | 47.47  |        |

Table S 6: Exciton coupling between benzaldehyde molecules of the cluster (in  $\text{cm}^{-1}$ ). Labels correspond to Figure 6a. The up-diagonal part corresponds to the exciton coupling computed using the transition density cube method (TDCM), while the low-diagonal part is computed in the ideal dipole approximation (IDA) using the transition dipole moments obtained by fitting the dynamic polarizability for each local charge density (LDT).

| Labels | 1      | 2      | 3      | 4      | 5     | 6      | 7      | 8     | 9     | 10     | 11     | 12    | 13     | 14     |
|--------|--------|--------|--------|--------|-------|--------|--------|-------|-------|--------|--------|-------|--------|--------|
| 1      |        | 104.10 | 48.73  | 40.97  | 21.08 | 15.83  | 47.24  | 29.23 | 17.71 | 72.05  | 136.50 | 31.45 | 12.91  | 12.22  |
| 2      | 214.16 |        | 22.08  | 14.24  | 12.26 | 5.48   | 20.89  | 34.21 | 7.06  | 31.22  | 31.46  | 17.25 | 8.38   | 14.90  |
| 3      | 30.61  | 36.66  |        | 5.93   | 6.34  | 55.25  | 14.83  | 12.73 | 49.75 | 1.23   | 69.30  | 1.96  | 6.87   | 4.95   |
| 4      | 26.26  | 9.21   | 51.12  |        | 29.10 | 37.61  | 7.01   | 4.73  | 56.77 | 1.07   | 14.72  | 16.89 | 23.25  | 6.31   |
| 5      | 54.31  | 15.39  | 4.63   | 96.78  |       | 110.73 | 12.28  | 6.35  | 17.51 | 13.36  | 13.47  | 86.29 | 111.23 | 7.10   |
| 6      | 185.43 | 37.82  | 100.10 | 114.27 | 44.68 |        | 57.98  | 16.30 | 73.76 | 13.58  | 10.84  | 30.35 | 2.62   | 1.15   |
| 7      | 59.64  | 33.79  | 18.33  | 7.75   | 25.87 | 43.49  |        | 31.02 | 32.83 | 32.38  | 37.78  | 8.48  | 92.00  | 69.26  |
| 8      | 28.52  | 44.61  | 111.67 | 19.34  | 4.02  | 32.22  | 146.61 |       | 22.40 | 21.08  | 47.02  | 3.63  | 9.20   | 45.14  |
| 9      | 20.40  | 9.50   | 54.55  | 17.91  | 45.71 | 60.53  | 35.96  | 42.83 |       | 6.42   | 4.06   | 2.97  | 81.49  | 12.57  |
| 10     | 213.40 | 70.71  | 0.40   | 6.26   | 9.64  | 17.67  | 52.41  | 15.61 | 1.84  |        | 28.93  | 19.87 | 9.61   | 164.50 |
| 11     | 88.52  | 156.03 | 35.18  | 5.62   | 6.72  | 24.43  | 74.95  | 13.18 | 5.73  | 293.34 |        | 7.94  | 13.83  | 58.73  |
| 12     | 99.67  | 17.88  | 17.06  | 13.86  | 31.31 | 41.82  | 34.35  | 13.25 | 17.78 | 41.56  | 33.71  |       | 34.90  | 13.46  |
| 13     | 21.40  | 13.26  | 15.83  | 30.75  | 96.15 | 45.24  | 254.74 | 1.16  | 44.68 | 25.10  | 39.70  | 63.85 |        | 34.70  |
| 14     | 14.66  | 1.54   | 11.60  | 5.70   | 6.05  | 12.59  | 176.34 | 38.60 | 12.92 | 219.36 | 50.35  | 9.16  | 41.79  |        |

## References

- (1) Becke, A. D. Density-functional exchange-energy approximation with correct asymptotic behavior. *Phys. Rev. A* **1988**, *38*, 3098–3100.
- (2) Perdew, J. P. Density-functional approximations for the correlation energy of the inhomogeneous electron gas. *Phys. Rev. B* **1986**, *33*, 8822–8824.
- (3) Grimme, S.; Ehrlich, S.; Goerigk, L. Effect of the damping function in dispersion corrected density functional theory. *J. Comput. Chem.* **2011**, *32*, 1456–1465.
- (4) Grimme, S.; Antony, J.; Ehrlich, S.; Krieg, H. A consistent and accurate ab initio parametrization of density functional dispersion correction (DFT-D) for the 94 elements H-Pu. *J. Chem. Phys.* **2010**, *132*, 154104.
- (5) Weigend, F.; Ahlrichs, R. Balanced Basis Sets of Split Valence, Triple Zeta Valence and Quadruple Zeta Valence Quality for H to Rn: Design and Assessment of Accuracy. *Phys. Chem. Chem. Phys.* **2005**, *7*, 3297–3305.
- (6) Eichkorn, K.; Treutler, O.; Öhm, H.; Häser, M.; Ahlrichs, R. Auxiliary basis sets to approximate Coulomb potentials. *Chem. Phys. Lett.* **1995**, *240*, 283–290.
- (7) Weigend, F. Accurate Coulomb-fitting basis sets for H to Rn. *Phys. Chem. Chem. Phys.* **2006**, *8*, 1057–1065.
- (8) Zheng, J.; Xu, X.; Truhlar, D. G. Minimally augmented Karlsruhe basis sets. *Theor. Chem. Acc.* **2011**, *128*, 295–305.
- (9) Perdew, J. P.; Burke, K.; Ernzerhof, M. Generalized Gradient Approximation Made Simple. *Phys. Rev. Lett.* **1996**, *77*, 3865–3868.
- (10) Perdew, J. P.; Burke, K.; Ernzerhof, M. Generalized Gradient Approximation Made Simple [Phys. Rev. Lett. 77, 3865 (1996)]. *Phys. Rev. Lett.* **1997**, *78*, 1396.
